# Supplementary material for: Direct Measurement of Curvature-Dependent Surface Tension in a Capillary-Condensed Alcohol Nanomeniscus
Source: arXiv:2010.04869 source file (2020-10-10)
Supplement: Supplementary file 1 [file Supplementary_Material_Jhe.pdf]

# Supporting Information: Direct Measurement of Curvature-Dependent Surface Tension in a Capillary-Condensed Alcohol Nanomeniscus

Dohyun Kim,[1] Jongwoo Kim,[2] Jonggeun Hwang,[1]
Dongha Shin,[1,3] Sangmin An,[1,4] and Wonho Jhe[1,*]

[1]*Center for 0D Nanofluidics, Institute of Applied Physics, Department of Physics and Astronomy, Seoul National University, Seoul 08826, Republic of Korea.*

[2]*Center for Convergent Research of Emerging Virus Infection, Korea Research Institute of Chemical Technology, Daejeon 34114, Republic of Korea.*

[3]*Division of Fine Chemistry and Engineering, College of Natural Science, Pai Chai University, Daejeon 35345, Republic of Korea.*

[4]*Department of Physics, Research Institute of Physics and Chemistry, Jeonbuk National University, Jeonju 54896, Korea.*

(Dated: October 7, 2020)

## SM 1. Materials and Methods

### *1. 1. Environment for measurement of critical distance*

To detect a single nucleation event by the force exerted by the nanomeniscus formed by liquid-vapor transition, an atomic force microscope (AFM) based on a quartz tuning fork (QTF) as a force sensor was employed like previous studies.[1–3] As a substrate for capillary condensation, an atomically flat muscovite mica (Grade V-1, SPI Supplies) was prepared by the tape-cleaving method.[4, 5] A fused quartz tip was pulled by mechanical puller (P-2000, Sutter Instrument),[5] which has a radius of curvature of about 30 $\sim$ 60 nm and a surface roughness of about 0.1 nm (rms) confirmed by analysis of scanning electron microscope image (Fig. S1) and the commercial AFM [5]. The tip attached on one prong of a QTF (C-002RX, EPSON) oscillated laterally with amplitude of $\sim$ 0.5 nm by applying sinusoidal voltage to the QTF at the resonance frequency of about 32,756 Hz by using a function generator (AMETEK).

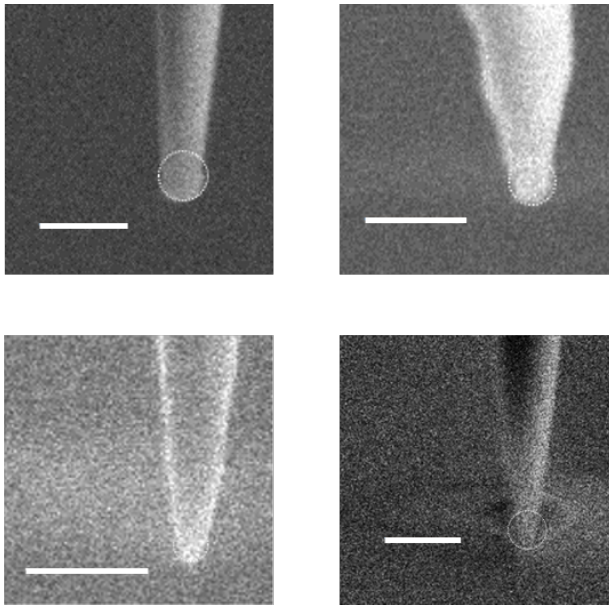

FIG. S1. Scanning electron microscope (SEM) images of the quartz tips used in the measurement. The scale bars indicate 200 nm. The contrast has been adjusted for clarity of the images.

An air-tight chamber was purged by the filtered, dehumidified (RH $<$ 0.1 ppm) nitrogen gas for at least 8 hours before experiments. Ethanol (absolute, $\geq$ 99.9%, Daejung) or *n*-propanol (HPLC grade, $\geq$ 99.9%, Sigma-Aldrich) was used to raise the saturation ratio

of the vapor pressure $p/p_0$ in the chamber to 0.1, 0.2, and 0.45 by controlling the ratio of the flow rate of alcohol-saturated nitrogen gas to that of pure nitrogen gas ($p/p_0 = 0$) using flow controllers (SFC5400, Sensirion). The alcohol liquid was freshly prepared for each experiment and the chamber was cleaned by wiping and drying after a set of experiment. Temperature inside the chamber was around 22.3 - 22.8°C and kept within ±0.1 °C measured by a temperature sensor (SHT85, Sensirion) during a set of measurement.

### *1. 2. Measurement of critical distance*

To detect the capillary condensation of alcohol and contact of the tip and substrate, the amplitude and phase signals of the QTF was monitored by a lock-in amplifier (AMETEK Signal Recovery). The tip approached and then retracted the mica surface after the contact by using a piezoelectric transducer (Fuji Ceramics co.) by $\sim 0.05$ nm at 500 ms interval. Typical amplitude-phase signals obtained during the approach-retraction cycle are in Fig. S2.

The critical distance $d_c$ was measured for 30 to 39 times for ethanol and 25 to 33 times for $n$-propanol vapor to get their histogram. The count data was fitted by Gaussian function in the histogram, and the average and standard deviation were obtained.

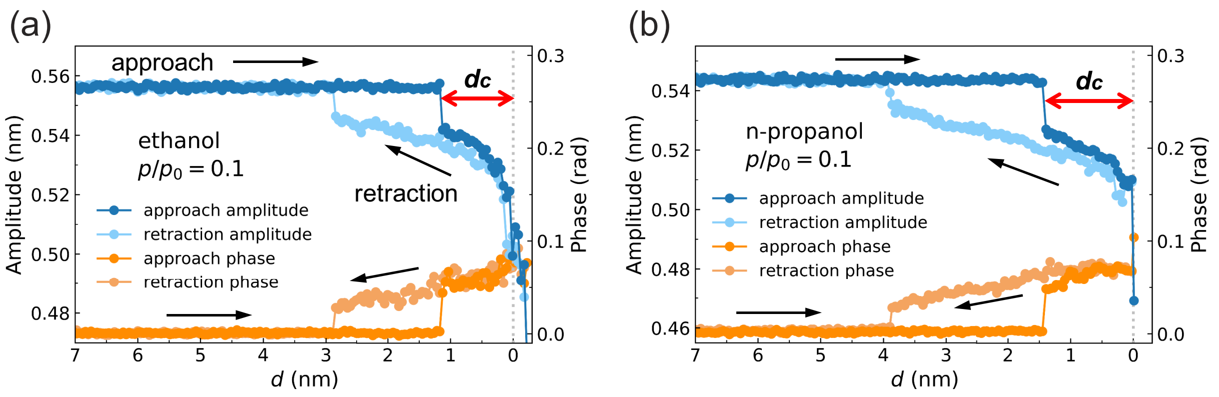


FIG. S2. (a) Typical amplitude-phase signals obtained during tip approach-retraction process for ethanol at $p/p_0 = 0.1$ and (b) for n-propanol at $p/p_0 = 0.1$. Hysteresis appears during retraction because the meniscus hardly evaporates during the tip retraction.

## SM 2. Geometry of the meniscus and the Young-Laplace equation

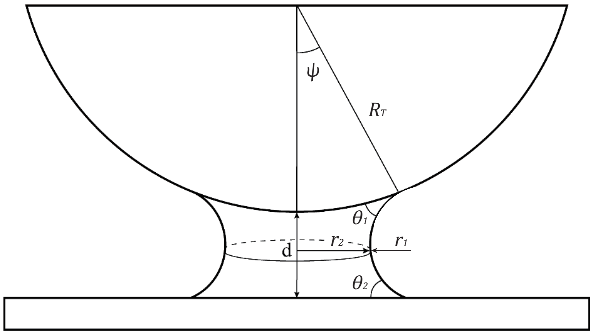


FIG. S3. Geometry of the nanomeniscus. The liquid-vapor interface of the nanomeniscus is in equilibrium having the constant mean curvature $1/R$ (=$1/r_1$+$1/r_2$). Here, $r_1$ and $r_2$ are the two principal radii-of-curvature (negative $r_1$ and positive $r_2$) and $d$ is the tip-surface distance. $\theta_1$ and $\theta_2$ are the contact angles, $R_\mathrm{T}$ the tip radius and $\psi$ the filling angle.

The relation between the curvature of the liquid-vapor interface and the pressure difference between two phases is described by the Young-Laplace equation by

$$\frac{1}{R} = \frac{d^2z/dr^2}{(1+(dz/dr)^2)^{3/2}} + \frac{dz/dr}{r(1+(dz/dr)^2)^{1/2}}, \tag{S1}$$

where $r$ is the horizontal axis and $z$ is the vertical axis of the meniscus [6]. The $1/R$ (=$1/r_1$+$1/r_2$) is a constant mean curvature where $r_1$ is negative ($\sim -1$ nm) and $r_2$ is positive ($\sim 10$ nm) in ambient condition of our experiment. The equation describes the surface of a constant mean curvature with respect to the symmetrical $z$-axis, the shape of a pendular ring as shown in Fig. S3. With the measured tip-surface critical distance $d_\mathrm{c}$, we find a solution of Eq. (S1) satisfying the boundary conditions (constant $\theta_1$, $\theta_2$ and $R_\mathrm{T}$) by solving numerically the elliptic integrals. Contact angles $\theta_1$ and $\theta_2$ are both assumed to be zero, the complete wetting, for the conservative analysis in present work.

With the given equilibrium curvature $1/R$, we are able to find the exact $d_\mathrm{max}$, beyond which there exists no solution. Notice that the equilibrium condition is assumed while the two surfaces approach for the distance measurements, since (i) the approach process is toward the condensed phase [7, 8] and (ii) the approaching two surfaces stay at a given distance long enough compared to the nucleation time during step-by-step approach [9].

Careful analysis of the experimental data, however, the measured $d_c$ is always larger than $d_{max}$ with a given curvature $1/R$ by the Kelvin equation assuming constant surface tension, especially at low $p/p_0$ (Fig. S4). Therefore, the curvature dependency of surface tension should be incorporated by a parameter $\delta$ that matches $d_{max}$ with the measured $d_c$.

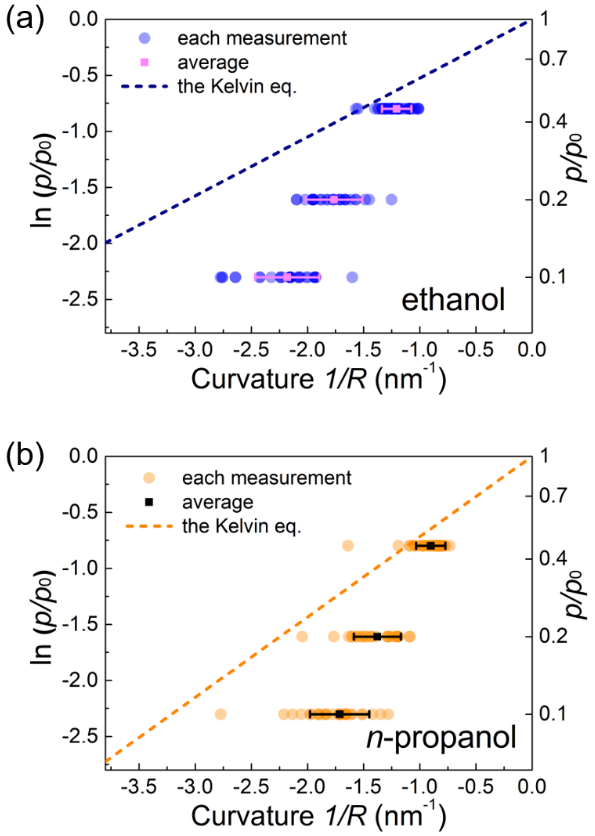


FIG. S4. Plot of $p/p_0$ versus the equilibrium curvature $1/R$. Scattered dots represent $1/R$ from each $d_c$ measurement for (a) ethanol and (b) propanol, whereas the dashed lines indicate prediction by the Kelvin equation that assumes the constant surface tension.

## SM 3. Consideration of errors in determination of surface tension

### *3. 1. Contamination of the tip or substrate*

To avoid the contamination of the tip and substrate, every corner of the chamber was wiped, dried, and being purged by the filtered clean $N_2$ gas when it was not used as well as overnight before each set of experiment adjusting $p/p_0$. Absence of contaminants was confirmed by scanning randomly selected areas on mica over a 1000 µm$^2$ [5].

In addition, when approaching the tip to the mica surface, we did not approach the tip further from the contact point ((iii) in Figs.1(e) and 1(f)) but quickly retreated the tip around the contact point, except when obtaining signals on Fig.1(f). As a result, we minimized the time and the area that the tip interacts with the liquid bridge formed as well as prevented plastic deformation and shape change of the tip due to mechanical hard contact. The SEM images of the quartz tip taken before and after measurement (Fig. S5) show that its shape and condition do not change unless it is contaminated. After use, the Energy Dispersive X-ray Spectroscopy (SEM-EDS) analysis can tell the contaminants on tip. Nevertheless, notice that when a sudden change occurs in the amplitude or phase signal of the freely oscillating QTF or when the rupture length of the meniscus becomes abnormally long, we replaced the tip immediately. For this reason, several different tips with similar apex radius are used even in one set of experiment, which broadens the $d_c$ distribution more than the water case due to the absence of such contamination issue for water [5]

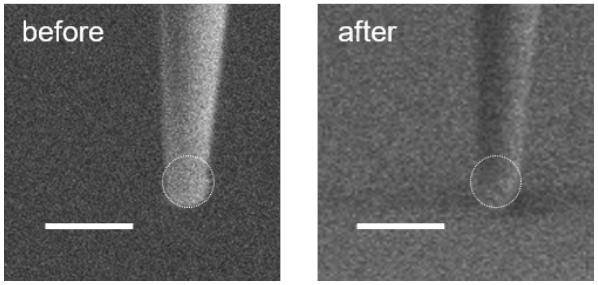


FIG. S5. Field emission-scanning electron microscopy (FE-SEM) images of the quartz tip takes before and after use, showing that the radius of curvature of the tip does not change much unless it is contaminated. The scale bars on the images are 200 nm. The contrast has been adjusted for clarity of the images.

*3. 2. The liquid film left over and pre-adsorbed on the mica surface*

To ensure the accuracy of $d_c$ measurement, it is necessary to address the effect of pre-adsorbed and leftover liquid films on the mica surface. It has been known that a thin film of one or two molecule thickness can be formed when mica is dipped in liquid alcohol and dried, or when placed in alcohol vapor close to saturation [10–12]. One layer thickness of ethanol (n-propanol) is about 0.47 nm (0.57 nm) [12, 13]. Although properties of such film formation are not known in unsaturated condition, $p/p_0$ lower than 0.5, we observe a thin liquid layer left over at the spot on mica where the tip-induced nucleation once occurs, even at $p/p_0$ as low as 0.1 for ethanol. It produces unwanted increase of $d_c$ in subsequent approach-condensation measurements on the same spot, which indicates that the molecules remaining on the surface form a liquid film without being evaporated even after waiting for several tens of minutes. The resulting systematic increase of $d_c$ is about one or two molecule thickness ($0.5 \sim 1$nm) as shown in Fig. S6 for the case of ethanol at $p/p_0 = 0.1$.

In some cases of approach with the film remaining, we found a sharp peak in the force-distance curve (Fig. S7), where the meniscus-induced interaction forces exerted on the tip are described by the damping coefficient $b_{\text{int}}$ and elastic constant $k_{\text{int}}$ [2]. Notice that it indicates that there exists a structured layer on the mica surface by one or two molecules thickness and also the layer is squeezed out as the tip makes step-by-step approach to the surface [10]. To avoid such systematic overestimation of $d_c$, each measurement is conducted at different locations of about 100 nm apart on mica.

In addition, because of the pre-adsorbed film, there are some cases that larger $d_c$ is measured even in the first trial at the spot. If the same thing happens around the spot, clearly indicating that there is a pre-adsorbed film around the spot, that specific measurement is excluded. Thereby, the $d_c$ values of pure condensation case are collected.

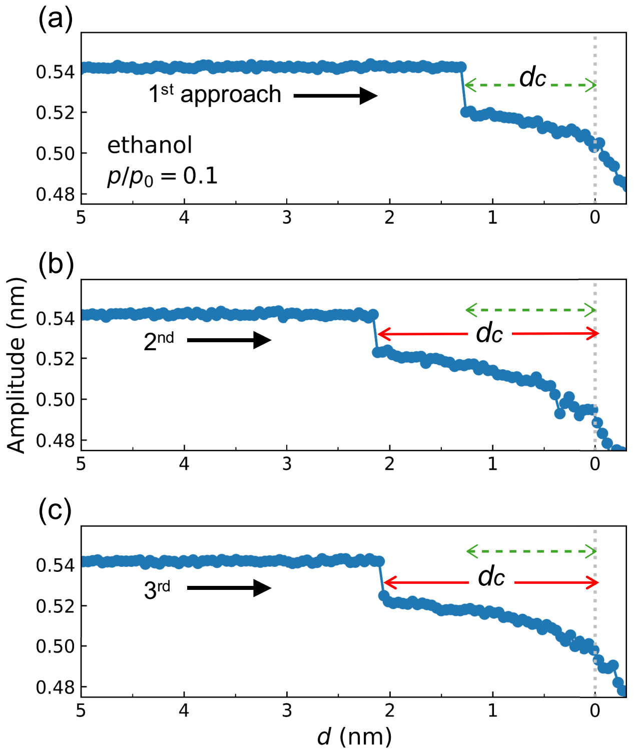


FIG. S6. Three consecutive trials of approach at the same point on the mica surface. Compared to the first trial (a), subsequent trials including the second (b) and the third (c) trial show a systematic increase in the measured $d_c$ by the size of one or two molecules.

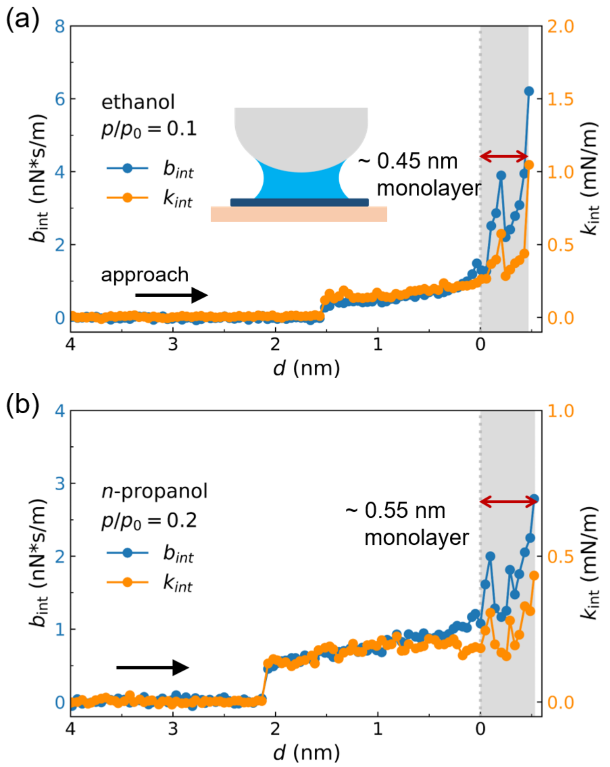


FIG. S7. (a) Liquid film of about $\sim$ 0.45 nm thickness (monolayer of ethanol) develops on mica even at $p/p_0 = 0.1$ for ethanol. Numerous approach-retractions are performed at a fixed vapor pressure ($p/p_0 = 0.1$, 0.2, 0.45) and a thin film remains even after one tip approach, lasting more than tens of minutes, which makes $d_c$ systematically larger by the film thickness. (b) For $n$-propanol, a film of about 0.55 nm thickness develops on mica.

### SM 4. Uncertainty of parameters used in the Kelvin equation and data analysis

The curvature dependent surface tension is characterized by the relation between the curvature $1/R$ of the curved liquid-vapor interface and the vapor pressure $p/p_0$ according to the Kelvin-Tolman equation in thermodynamic equilibrium. Therefore, to be accurate, the parameters used in the calculations should be carefully addressed for quantitative analysis of the surface tension. A detailed and quantitative analysis of the possible errors that are associated with, for example, the tip radius, change in the molecular density and adjustment of $p/p_0$, is provided in this section. In summary, the very conservative error estimates lead to deviation of $\delta$ by as much as $-33\%$ up to $+78\%$, nonetheless the sign of $\delta$ itself is invariant.

Firstly, the vapor pressure $p/p_0$ in the chamber is slightly different from the expected. The nitrogen gas is assumed to be saturated at $p/p_0 = 1$ and used to control $p/p_0$ inside the chamber using dehumidified gas. However, there can be an error in the vapor pressure. Assuming that the vapor pressure $p/p_0$ of the nitrogen gas varies 10% increase or decrease in each vapor pressure. Table I shows how the Tolman length $\delta$ changes according to the variation. We found that the error in the vapor pressure can lead to an error in the Tolman length $\delta$ up to $\pm 33\%$.

| $p/p_0$ | $\delta_{\text{ethanol}}$ (nm) | $\delta_{\text{propanol}}$ (nm) |
|---|---|---|
| 0.09 | 0.24 | 0.29 |
| 0.10 | 0.23 | 0.27 |
| 0.11 | 0.22 | 0.26 |
| 0.182 | 0.26 | 0.31 |
| 0.20 | 0.24 | 0.28 |
| 0.215 | 0.23 | 0.26 |
| 0.42 | 0.23 | 0.28 |
| 0.45 | 0.17 | 0.21 |
| 0.475 | 0.13 | 0.14 |

TABLE I. The error associated with the pressure ratio. We assume the pressure of $N_2$ gas varies as $p/p_0 = 0.9 \sim 1.1$, even if the saturated gas is obtained at $p/p_0 = 1$ and put into the chamber to adjust the saturation ratio inside the chamber.

Secondly, radius of the tip and contact angle at three phase (liquid-vapor-solid) contact line, which serve as a boundary condition to determine the curvature $1/R$ from the critical distance of nucleation $d_{\mathrm{c}}$, should be addressed.

Due to the resolution limit of SEM image for the quartz tip, the tip-radius measurement suffers from inevitable ambiguity. However, even if we set the error of the tip radius $R_{\mathrm{T}}$ large enough, it does not much affect the values of $\delta$ (TABLE II).

Furthermore, the microscopic contact angles at the three phase contact line on the tip and mica may differ from the macroscopic measurement and may be affected by the oscillation of the tip. Varying the error of the contact angles from $0°$ to $30°$ for the tip and from $0°$ to $10°$ for the mica, we estimate up to 78% larger value of $\delta$, which nonetheless does not change its sign (TABLE II). The effect of the tip oscillation on the nucleation and $d_{\mathrm{c}}$ measurement can be negligible, as the oscillating amplitude ( 0.5 nm) is small enough compared to the lateral size of the meniscus ($\sim 10$ nm) and the oscillation period is longer than the relaxation time of the confined molecules. Our previous study showed that the results of $d_{\mathrm{c}}$ measurements are not affected as the amplitude changes in a range smaller than 1 nm [5].

Finally, since we assume the ideal gas and incompressible liquid, the related nonidealities can be also considered by varying the molecular volume $v_l$. We estimate $\pm 20\%$ of change in $v_{l,bulk}$ gives about $\pm 22\%$ errors in $\delta$ (see TABLE II).

| Variable | $R_{\mathrm{tip}}$ (nm) | $\theta_{\mathrm{tip}}$ (°) | $\theta_{\mathrm{substrate}}$ (°) | $v_{\mathrm{l}}$ ($\mathrm{m}^3$) | $\delta$ (nm) |
|---|---|---|---|---|---|
| This work | 45 | 0 | 0 | $v_{\mathrm{l,bulk}}{}^*$ | 0.23 |
| Tip radius | 30 | 0 | 0 | $v_{\mathrm{l,bulk}}{}^*$ | 0.25 |
| $R_{\mathrm{tip}}$ | 60 | 0 | 0 | $v_{\mathrm{l,bulk}}{}^*$ | 0.22 |
| Contact angles $\theta_{\mathrm{tip}}$, $\theta_{\mathrm{substrate}}$ | 45 | 0 | 10 | $v_{\mathrm{l,bulk}}{}^*$ | 0.27 |
| | 45 | 10 | 0 | $v_{\mathrm{l,bulk}}{}^*$ | 0.27 |
| | 45 | 10 | 10 | $v_{\mathrm{l,bulk}}{}^*$ | 0.3 |
| | 45 | 20 | 10 | $v_{\mathrm{l,bulk}}{}^*$ | 0.35 |
| | 45 | 30 | 10 | $v_{\mathrm{l,bulk}}{}^*$ | 0.41 |
| Molecular volume | 45 | 0 | 0 | 0.8 $v_{\mathrm{l,bulk}}{}^*$ | 0.28 |
| $v_{\mathrm{l}}$ | 45 | 0 | 0 | 1.2 $v_{\mathrm{l,bulk}}{}^*$ | 0.19 |

For ethanol, $p/p_0 = 0.1$. $^*v_{\mathrm{l,bulk}} = 9.76 \times 10^{-29}$ $\mathrm{m}^3$

TABLE II. The errors estimated for possible sources of error.

### SM 5. Second-order curvature effect in the Tolman equation

Recent works on the analysis of the homogeneous nucleation (HON) experiment data suggested the use of the second order expansion of the surface tension in terms of the curvature $1/R$ when incorporating the curvature correction of surface tension [14, 15], beyond the first order expansion that is based on the constant Tolman length. The second order expansion includes the curvature dependence of the Tolman length itself, approximated as follows [16],

$$\delta\left(\frac{1}{R}\right) = \delta_\infty + \frac{\alpha}{2R}, \tag{S2}$$

where $1/R$ is the mean curvature ($= 1/r_1 + 1/r_2 = 2/R_s$ in case of a sphere of radius $R_s$) defined on the surface of tension, $\delta_\infty$ is the curvature independent term and $\alpha$ is the coefficient of the second term. Putting Eq. S2 into the Gibbs-Tolman-Koenig-Buff (GTKB) equation, integrating and Taylor expanding it to the second order of $1/R$, one can get the curvature dependence of surface tension as follows [16],

$$\frac{\sigma_0}{\sigma} = 1 + \frac{\delta_\infty}{R} + \frac{(\delta_\infty^2 + \alpha)}{4R^2}. \tag{S3}$$

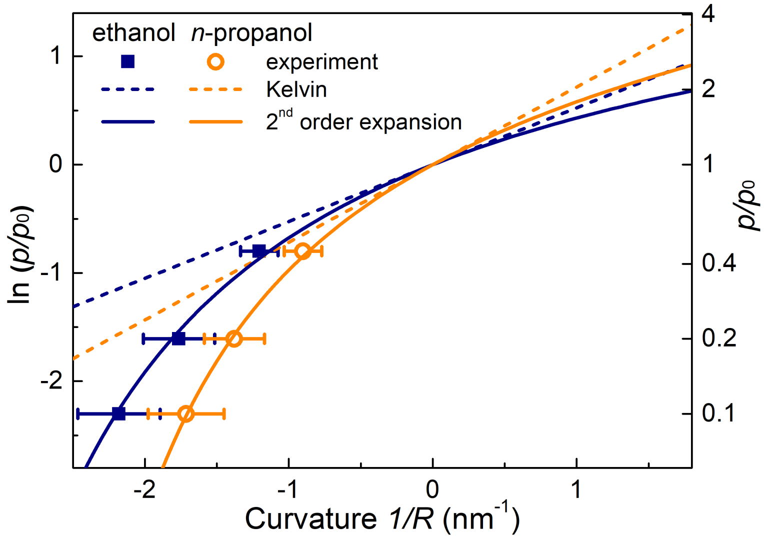


FIG. S8. Fitting our data with Eq. S3, we obtain $\delta_\infty = 0.22\,\mathrm{nm}$ and $\delta_\infty^2 + \alpha = -0.022\,\mathrm{nm}^2$ for ethanol and $\delta_\infty = 0.25\,\mathrm{nm}$ and $\delta_\infty^2 + \alpha = -0.057\,\mathrm{nm}^2$ for n-propanol.

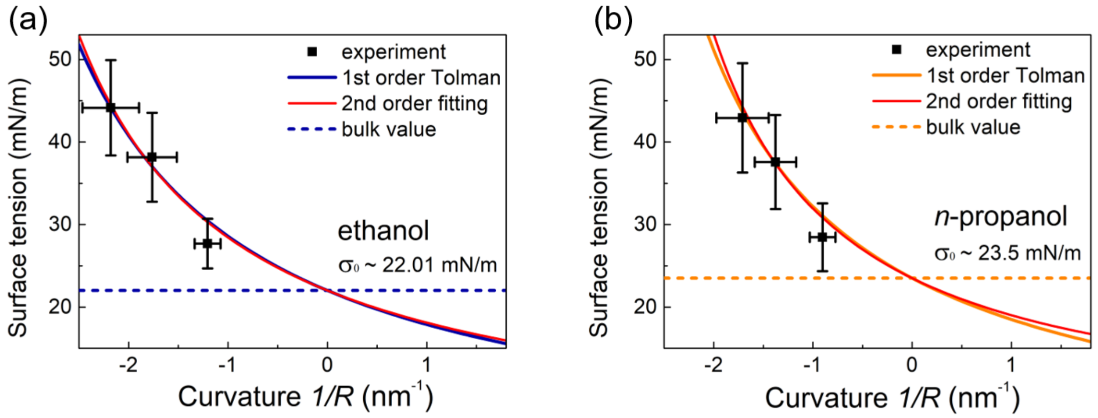


FIG. S9. Surface tension incorporating the curvature correction with the Tolman length $\delta$ for (a) ethanol and (b) n-propanol. The red curves represent the fitting with the second-order expansion of surface tension in terms of $1/R$

This equation incorporates the spherical rigidity, referred to as the Helfrich coefficient $k_s$ $= (3\delta_\infty^2 - \alpha)\sigma_0$, as well as the curvature-independent Tolman length $\delta_\infty$ as the free parameter. Fitting Eq. S3 to our experimental data yields $\delta_\infty = 0.22\,\text{nm}$ and $\delta_\infty^2 + \alpha = -0.022\,\text{nm}^2$ for ethanol, in good agreement with the results of HON [14, 17] (See Fig. 4 and Fig. S9 of reference [14]). For n-propanol, $\delta_\infty = 0.25\,\text{nm}$ and $\delta_\infty^2 + \alpha = -0.057\,\text{nm}^2$, as plotted by the red curves in Fig. S8. The corresponding surface tension values versus the curvature $1/R$ are presented in Fig. S9.

The Tolman length is defined as the difference between the surface of tension, and the surface of vanishing superficial density for which the assumption of uniform density for the two bulk phases divided by this zero-thickness surface gives the exactly same mass of the pure fluid in each phase as in real situation [18, 19]. Therefore, the value of the Tolman length is closely related to intermolecular distance and interaction range [20], sensitively depending on the temperature and type of molecule.

Let us emphasize again that our measurements show the dominant role of curvature-dependent surface tension becomes in the initial stage of nucleation, which should be considered up to the second order for more accurate characterization, when describing the nucleation processes such as condensation, cavitation or adsorption.

## SM 6. Curvature effect in other HEN rate-measurement experiment

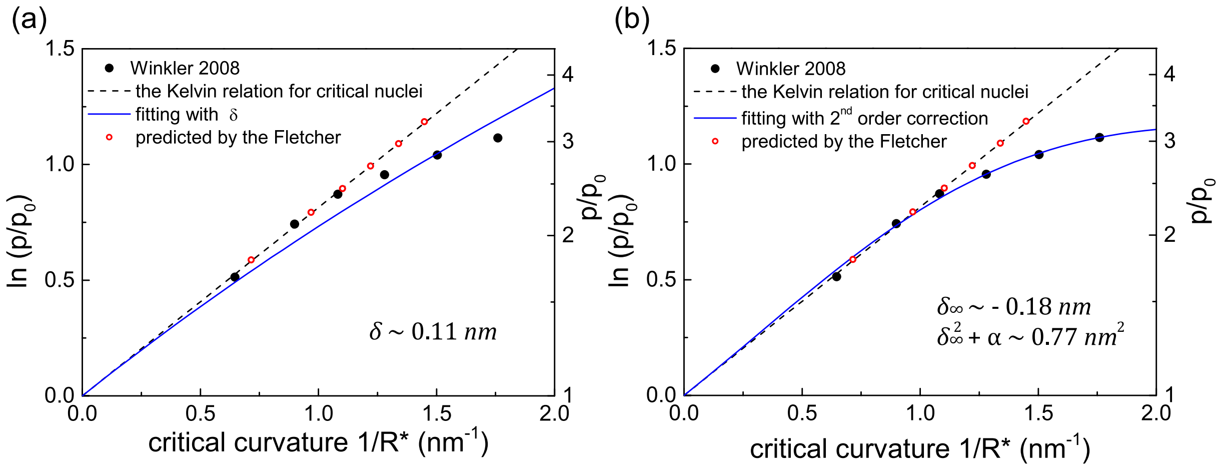


FIG. S10. The curvature-dependent surface tension is employed to the results of the HEN experiment of Ref.[21]. (a) Fitting with $\delta = 0.11\,\mathrm{nm}$, which has the same positive sign but deviates from the first-order fitting as the curvature increases. (b) Fitting with the second-order correction of surface tension gives $\delta_\infty = -0.18\,\mathrm{nm}$ and $\delta_\infty^2 + \alpha = 0.77\,\mathrm{nm}^2$, which shows excellent agreement.

Unlike in HON studies, the curvature-dependent surface tension has not been incorporated in HEN studies. The HEN studies focus more on the liquid-solid interface or three phase (liquid-vapor-solid) contact line rather than the LV interface because they are mainly interested in the activation properties of the seed particles which provide the nucleation site [21, 22]. The results of HEN rate measurement in supersaturated $n$-propanol vapor with the seed particles down to $\sim 1\,\mathrm{nm}$ in diameter are presented in Ref. [21]. The Fletcher theory is employed to analyze the results, which predicts the onset saturation ratio ($S_F$) slightly larger than the measured onset ratio ($S_{\mathrm{measured}}$). Here, we suggest that if the curvature dependence of surface tension is incorporated, the expected and measured results are in good agreement. Fig. S10 shows the results that are fitted with the constant Tolman length as well as with the second-order expansion.

From the explanation given in Ref. [21] that the ratio of the experimental activation diameter of the seed particle ($D_{\mathrm{p}}$) to the Kelvin diameter ($D_{\mathrm{k}} = 2r_{\mathrm{k}}$) is almost size-independent as around 0.65, the predicted LV interface curvature of the critical nucleus ($1/R_{\mathrm{F}}^* = 2/r_{\mathrm{k}}$) can be set. Then, we establish the equation for the nucleation probability $P(S)$, giving $P(S_{\mathrm{F}}) = 1/2$ with the critical curvature $1/R_{\mathrm{F}}^*$. With the equation $P(S)$, the constant Tol-

man length $\delta$ is determined, from which the equation for the nucleation probability provides $P(S_{\text{measured}}) = 1/2$ for each $S_{\text{measured}}$. Finally, the value of $1/R^*$ is obtained by employing the Kelvin-Tolman equation (Eq. S3) with each $\delta$ and $S_{\text{measured}}$. The values of $1/R^*$ and the corresponding $S_{\text{measured}}$ are plotted and fitted with a constant $\delta$ in Fig. S10(a), which shows deviation with the increase of curvature. The resulting Tolman length $\delta$ exhibits the same sign and the similar value compared to our results, implying the similar behavior of surface tension change that the larger positive (negative) curvature $1/R$ has the smaller (larger) surface tension than bulk. Meanwhile, the second-order expansion fitting shows the better agreement with the experiment as shown in Fig. S10(b). Notice that the measured onset saturation ratio $S_{\text{measured}}$ and the predicted ration by the Fletcher theory $S_{\text{F}}$ are from Fig. 2 of Ref. [21]. The kinetic pre-factor and some thermodynamic parameters needed for model calculation are all from the Supporting Online Material of the same reference.

* corresponding author.whjhe@snu.ac.kr

[1] H. Choe, M.-H. Hong, Y. Seo, K. Lee, G. Kim, Y. Cho, J. Ihm, and W. Jhe, Phys. Rev. Lett. **95**, 187801 (2005).

[2] M. Lee, J. Jahng, K. Kim, and W. Jhe, Appl. Phys. Lett. **91**, 023117 (2007).

[3] M. Lee, B. Kim, J. Kim, and W. Jhe, Nat. Commun. **6**, 7359 (2015).

[4] J. Israelachvili, N. Alcantar, N. Maeda, T. Mates, and M. Ruths, Langmuir **20**, 3616 (2004).

[5] S. Kim, D. Kim, J. Kim, S. An, and W. Jhe, Phys. Rev. X **8**, 041046 (2018).

[6] F. Orr, L. Scriven, and A. Rivas, J. Fluid Mech. **67**, 723 (1975).

[7] E. Sahagún, P. García-Mochales, G. M. Sacha, and J. J. Sáenz, Phys. Rev. Lett. **98**, 176106 (2007).

[8] Y. Men, X. Zhang, and W. Wang, J. Chem. Phys. **131**, 184702 (2009).

[9] R. Szoszkiewicz and E. Riedo, Phys. Rev. Lett. **95**, 135502 (2005).

[10] S. Loi, G. Sun, V. Franz, and H.-J. Butt, Phys. Rev. E **66**, 031602 (2002).

[11] L. Wang, Y. Song, B. Zhang, and E. Wang, Thin Solid Films **458**, 197 (2004).

[12] P. Bampoulis, J. P. Witteveen, E. S. Kooij, D. Lohse, B. Poelsema, and H. J. W. Zandvliet, ACS Nano **10**, 6762 (2016).

[13] M. L. Gee, T. W. Healy, and L. R. White, J. Colloid Interface Sci. **133**, 514 (1989).

[14] N. Bruot and F. Caupin, Phys. Rev. Lett. **116**, 056102 (2016).

[15] A. Aasen, D. Reguera, and O. Wilhelmsen, Phys. Rev. Lett. **124**, 045701 (2020).

[16] V. G. Baidakov and K. S. Bobrov, J. Chem. Phys. **140**, 184506 (2014).

[17] R. Strey, P. E. Wagner, and T. Schmeling, J. Chem. Phys. **84**, 2325 (1986).

[18] R. Tolman, J. Chem. Phys. **16**, 758 (1948).

[19] R. Tolman, J. Chem. Phys. **17**, 333 (1949).

[20] Y. Lei, T. Bykov, S. Yoo, and X. Zeng, J. Am. Chem. Soc. **127**, 15346 (2005).

[21] P. Winkler, G. Steiner, A. Vrtala, H. Vehkamäki, M. Noppel, K. Lehtinen, G. Reischl, P. Wagner, and M. Kulmala, Science **319**, 1374 (2008).

[22] A. I. Hienola, P. M. Winkler, P. E. Wagner, H. Vehkamäki, A. Lauri, I. Napari, and M. Kulmala, J. Chem. Phys. **126**, 094705 (2007).
